# Supplementary material for: Localizing Moments in Long Video Via Multimodal Guidance
Source: arXiv:2302.13372 source file (2023-10-15)
Supplement: Supplementary file 2 [file 06-appendix-tab3.tex]

% Please add the following required packages to your document preamble:
% \usepackage{booktabs}
% \usepackage{multirow}
\begin{table*}[!t]
%\vspace{-14.8cm}

\centering
\setlength{\tabcolsep}{2.5pt}
 
%\vspace{-17.5cm}
%\centering
\resizebox{\linewidth}{!}{%
\footnotesize
%\rotatebox{90}
\begin{tabular}{@{}ccccccccccccccccc@{}}
\toprule
\textbf{} &
  \textbf{} &
  \multicolumn{3}{c}{\textbf{R@1}} &
  \multicolumn{3}{c}{\textbf{R@5}} &
  \multicolumn{3}{c}{\textbf{R@10}} &
  \multicolumn{3}{c}{\textbf{R@50}} &
  \multicolumn{3}{c}{\textbf{R@100}} \\ \midrule
\textbf{Model} &
  \textbf{Query} &
  \textbf{IoU=0.1} &
  \textbf{IoU=0.3} &
  \textbf{IoU=0.5} &
  \textbf{IoU=0.1} &
  \textbf{IoU=0.3} &
  \textbf{IoU=0.5} &
  \textbf{IoU=0.1} &
  \textbf{IoU=0.3} &
  \textbf{IoU=0.5} &
  \textbf{IoU=0.1} &
  \textbf{IoU=0.3} &
  \textbf{IoU=0.5} &
  \textbf{IoU=0.1} &
  \textbf{IoU=0.3} &
  \textbf{IoU=0.5} \\ \midrule
\multirow{3}{*}{Zero-shot CLIP} &
  \xmark &
  $6.65$ &
  $3.19$ &
  $1.35$ &
  $14.80$ &
  $9.88$ &
  $5.31$ &
  $19.79$ &
  $13.84$ &
  $8.03$ &
  $36.30$ &
  $27.47$ &
  $18.06$ &
  $45.59$ &
  $35.33$ &
  $23.93$ \\ %\cmidrule(l){2-17} 
 &
  AG &
  $5.64$ &
  $2.89$ &
  $1.28$ &
  $13.79$ &
  $9.43$ &
  $5.19$ &
  $18.88$ &
  $13.22$ &
  $7.89$ &
  $\mathbf{37.88}$ &
  $26.90$ &
  $17.34$ &
  $\mathbf{46.61}$ &
  $36.60$ &
  $24.12$ \\ %\cmidrule(l){2-17} 
 &
  DE &
  $\mathbf{9.05}$ &
  $\mathbf{4.52}$ &
  $\mathbf{2.01}$ &
  $\mathbf{18.00}$ &
  $\mathbf{12.60}$ &
  $\mathbf{7.14}$ &
  $\mathbf{22.76}$ &
  $\mathbf{16.83}$ &
  $\mathbf{10.65}$&
  $37.24$ &
  $\mathbf{30.13}$ &
  $\mathbf{21.75}$ &
  $44.37$ &
  $\mathbf{37.02}$ &
  $\mathbf{27.76}$ \\ \midrule
\multirow{3}{*}{VLG-Net} &
  \xmark &
  $3.43$ &
  $2.56$ &
  $1.49$ &
  $11.32$ &
  $8.92$ &
  $5.54$ &
  $17.19$ &
  $13.92$ &
  $9.01$ &
  $37.80$ &
  $32.38$ &
  $22.93$ &
  $48.63$ &
  $42.34$ &
  $31.34$ \\ %\cmidrule(l){2-17} 
 &
  AG &
  $3.89$ &
  $2.82$ &
  $1.70$ &
  $14.31$ &
  $9.30$ &
  $7.12$ &
  $18.69$ &
  $15.24$ &
  $9.87$ &
  $39.37$ &
  $35.22$ &
  $24.00$ &
  $49.87$ &
  $44.19$ &
  $34.16$ \\ %\cmidrule(l){2-17} 
 &
  DE &
  $\mathbf{5.37}$ &
  $\mathbf{4.01}$ &
  $\mathbf{2.31}$ &
  $\mathbf{15.52}$ &
  $\mathbf{12.56}$ &
  $\mathbf{8.16}$ &
  $\mathbf{22.37}$ &
  $\mathbf{18.58}$ &
  $\mathbf{12.57}$ &
  $\mathbf{42.58}$ &
  $\mathbf{37.33}$ &
  $\mathbf{28.14}$ &
  $\mathbf{52.72}$ &
  $\mathbf{46.44}$ &
  $\mathbf{36.46}$ \\ \midrule
\multirow{3}{*}{Moment-DETR} &
  \xmark &
  $0.28$ &
  $0.20$ &
  $0.12$ &
  $1.44$ &
  $1.07$ &
  $0.62$ &
  $2.62$ &
  $1.87$ &
  $1.05$ &
  $10.41$ &
  $7.61$ &
  $4.47$ &
  $18.21$ &
  $13.18$ &
  $7.93$ \\ %\cmidrule(l){2-18} 
 &
  AG &
  $0.65$ &
  $0.59$ &
  $0.36$ &
  $2.11$ &
  $1.78$ &
  $1.02$ &
  $4.54$ &
  $2.83$ &
  $1.45$ &
  $18.44$ &
  $14.22$ &
  $8.32$ &
  $32.34$ &
  $22.97$ &
  $12.54$ \\ %\cmidrule(l){2-17} 
 &
  DE &
  $\mathbf{4.84}$ &
  $\mathbf{3.69}$ &
  $\mathbf{2.17}$ &
  $\mathbf{15.34}$ &
  $\mathbf{11.95}$ &
  $\mathbf{7.25}$ &
  $\mathbf{22.80}$ &
  $\mathbf{17.99}$ &
  $\mathbf{10.93}$ &
  $\mathbf{46.01}$ &
  $\mathbf{37.10}$ &
  $\mathbf{22.62}$ &
  $\mathbf{57.06}$ &
  $\mathbf{46.19}$ &
  $\mathbf{28.09}$ \\ \bottomrule
\end{tabular}
}

\vspace{-.1cm}
\caption{\label{tab:agnosti}{\bf Describable windows (full metrics).} In this table, we report Recall@$K$ on the validation partition of MAD for the baseline models under three settings: without any guidance (rows 1, 4, and 7), with query agnostic guidance (AG), and with query dependent guidance (DE). All three baselines benefit from using query-dependent guidance, while zero-shot CLIP is the only model negatively impacted by using query-agnostic guidance. We conclude that the language queries are indispensable for the Guidance Model, as they help reduce the search space for the grounding task.
\vspace{-.3cm}}
\end{table*}
